# Supplementary material for: Performance Analysis of Semi-Persistent Scheduling Throughput in 5G NR-V2X: A MAC Perspective
Source: arXiv:2208.10653 source file (2022-08-23)
Supplement: Supplementary file 1 [file appendix.tex]

% \subsection{Appendix 1}\label{app:1}
